# Supplementary material for: From many-body oscillations to thermalization in an isolated spinor gas
Source: arXiv:2010.13832 ancillary file (2020-12-18)
Supplement: Supplementary file 1 [file Supplemental.pdf]

# Supplemental Material:

## From many-body oscillations to thermalization in an isolated spinor gas

Bertrand Evrard, An Qu, Jean Dalibard and Fabrice Gerbier

*Laboratoire Kastler Brossel, Collège de France, CNRS,*

*ENS-PSL Research University, Sorbonne Université,*

*11 Place Marcelin Berthelot, 75005 Paris, France*

(Dated: December 17, 2020)

### I. ENERGY SCALES AND SPECTRUM

We recall the total Hamiltonian describing our spinor BEC within the single mode approximation

$$\hat{H} = q(\hat{N}_{+1} + \hat{N}_{-1}) + \frac{U_s}{2N} \hat{S}^2, \quad (1)$$

with

$$\begin{aligned} \hat{S}^2 = N + \hat{N}_0 + 2\hat{N}_0(N - \hat{N}_0) + \hat{S}_z^2 \\ + 2(\hat{a}_{+1}^\dagger \hat{a}_{-1}^\dagger \hat{a}_0^2 + \hat{a}_0^{\dagger 2} \hat{a}_{+1} \hat{a}_{-1}). \end{aligned} \quad (2)$$

In our experiment, we studied the evolution after a quench of the quadratic Zeeman energy  $q$  of a polar BEC [1], where each atom initially occupies the  $|m=0\rangle$  Zeeman state. The energy  $E_i \approx U_s$  of the initial state originates solely from the interaction term. Given that the energy cost to produce a pair of atoms in  $(+1, -1)$  state is  $2q$ , we can distinguish three regimes depending on the value of  $q$  after the quench :

- (i)  $q \gg U_s$  : we expect essentially no evolution of the initial state, which is very close to the ground state of the system.
  - (ii)  $U_s/N \ll q \ll U_s$  : the BEC is weakly depleted, and the dynamics of a polar BEC is well captured by the Bogoliubov approach (see Sec. II). In an energy window around  $E_i$ , the many-body spectrum  $n\hbar\omega_B$  with  $n$  an integer is almost linear with the quantum number  $n$  (the number of excitation quanta).
  - (iii)  $\frac{U_s}{N^2} \ll q \ll U_s/N$  : in that case the QZE is negligible compared to the energy  $E_i$  of the initial state and can thus be omitted. The spectrum is now quadratic with the quantum number  $S$  (the total spin angular momentum), leading to overdamped dynamics.
- For completeness, we mention the existence of a fourth regime, not relevant for the dynamics of a polar BEC, but for the lowest energy states.
- (iv)  $q \ll U_s/N^2$  : the QZE is small compared to the smallest gap (between the ground state and the first excited state) of the interaction Hamiltonian. Thus, the QZE can be neglected for all eigenstates, not only for the relatively high energy ones that we are considering in our experiment.

These four regimes are sketched in figure 1, with a table of the experimental parameters. In figure 2, we present an exact diagonalization of the Hamiltonian (1).

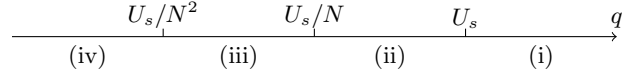

FIG. 1. Energy scales for a spin-1 BEC with zero magnetization in the SMA.

| Data set | $q/\hbar$ [Hz] | $U_s/\hbar$ [Hz] | $N$       | $Nq/U_s$ |
|----------|----------------|------------------|-----------|----------|
| 1        | 2.00(1)        | 17.5(1.4)        | 5700(600) | 650      |
| 2        | 1.00(1)        | 17.5(1.4)        | 5400(700) | 300      |
| 3        | 0.31(1)        | 17.5(1.4)        | 5400(700) | 96       |
| 4        | 0.05(1)        | 17.5(1.4)        | 5100(700) | 14.5     |
| 5        | 0.30(1)        | 16(2)            | 274(40)   | 5.2      |
| 6        | 0.14(1)        | 16(2)            | 287(43)   | 2.5      |
| 7        | 0.011(2)       | 64(7)            | 835(54)   | 0.14     |
| 8        | 0.011(2)       | 24(3)            | 230(24)   | 0.11     |
| 9        | 0.011(2)       | 17(2)            | 107(15)   | 0.070    |

TABLE I. Experimental parameters for the data presented in the paper. The data sets 1  $\rightarrow$  4 correspond to regime (ii) and are used in figure 3 of the Supplemental. Data set 3 is used in the figure 1 of the main text. Data sets 7  $\rightarrow$  9 correspond to regime (iii) and are used in the figure 2 of the main text. All data sets, including 5 & 6 taken at the crossover from (i) to (iii), are compared to the GGE predictions in figure 4 of the Supplemental (see Sec. II B). The interaction strength  $U_s$  is calibrated using a fit of the oscillation of  $N_p$  given Eq.(12). It depends of  $N$  and on the trap frequencies.

### II. BOGOLIUBOV REGIME

For  $q \gg U_s/N$  [regimes (i) and (ii)], the condensate is weakly depleted, and the Bogoliubov approximation leads to the quadratic Hamiltonian

$$\begin{aligned} \hat{H}_B = (q + U_s) (\hat{N}_{+1} + \hat{N}_{-1}) + U_s (\hat{a}_{+1} \hat{a}_{-1} + \hat{a}_{+1}^\dagger \hat{a}_{-1}^\dagger) \\ + U_s, \end{aligned} \quad (3)$$

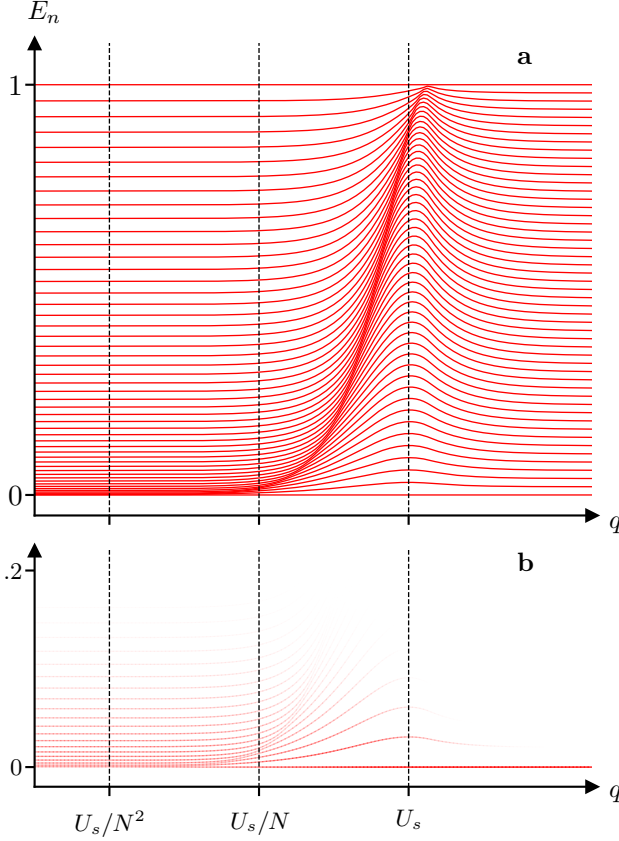

FIG. 2. (a) Spectrum of the Hamiltonian (1), for  $N = 100$  and  $S_z = 0$  versus the QZE  $q$  (in log scale). The energies  $E_n(q)$  are rescaled for each value of  $q$  so that the energy of the ground state  $E_{\min}$  and of the most excited state  $E_{\max}$  are constant. The initial state  $|\psi\rangle = |m = 0\rangle^{\otimes N}$  belongs to the low energy sector. In (b) we zoom on this section, and here the brightness of the line  $E_n(q)$  is proportional to  $\langle n(q)|\psi_i\rangle$ , with  $|n(q)\rangle$  the energy eigenstates. For  $U_s/N \ll q$ , the relevant part of the spectrum is almost linear, while for  $q \lesssim U_s/N$  it is essentially quadratic.

up to terms of order  $1/N$ . We introduce the Bogoliubov operators

$$\hat{\alpha} = \cosh(\theta)\hat{a}_{+1} - \sinh(\theta)\hat{a}_{-1}^{\dagger}, \quad (4)$$

$$\hat{\beta} = \sinh(\theta)\hat{a}_{+1}^{\dagger} - \cosh(\theta)\hat{a}_{-1}, \quad (5)$$

with

$$\cosh(2\theta) = \frac{q + U_s}{\hbar\omega_B} \quad \text{and} \quad \sinh(2\theta) = -\frac{U_s}{\hbar\omega_B}, \quad (6)$$

and the Bogoliubov energy  $\hbar\omega_B = \sqrt{q(q + 2U_s)}$ . This transformation diagonalizes the Hamiltonian (3),

$$\hat{H}_B = \hbar\omega_B[\hat{\alpha}^{\dagger}\hat{\alpha} + \hat{\beta}^{\dagger}\hat{\beta} - 2\sinh^2(\theta)] + U_s. \quad (7)$$

The number of pairs  $\hat{N}_p = (\hat{N}_{+1} + \hat{N}_{-1})/2$  can be written as a function of the Bogoliubov modes

$$\hat{N}_p = \frac{\cosh(2\theta) - 1}{2} + \frac{\cosh(2\theta)}{2} (\hat{\alpha}^{\dagger}\hat{\alpha} + \hat{\beta}^{\dagger}\hat{\beta}) - \frac{\sinh(2\theta)}{2} (\hat{\alpha}^{\dagger}\hat{\beta}^{\dagger} + \hat{\alpha}\hat{\beta}). \quad (8)$$

The magnetization along  $z$  is given by

$$\hat{S}_z = \hat{\alpha}^{\dagger}\hat{\alpha} - \hat{\beta}^{\dagger}\hat{\beta}. \quad (9)$$

### A. Dynamics

The time evolution of the Bogoliubov operators in the Heisenberg picture is straightforward, for instance  $\hat{\alpha}(t) = \exp(-i\omega_B t)\hat{\alpha}(0)$ . For our initial state  $|m = 0\rangle^{\otimes N}$ , we have

$$\langle \hat{\alpha}^{\dagger}\hat{\alpha} \rangle_i = \langle \hat{\beta}^{\dagger}\hat{\beta} \rangle_i = \sinh^2(\theta), \quad (10)$$

$$\langle \hat{\alpha}\hat{\beta} \rangle_i = \frac{1}{2} \sinh(2\theta). \quad (11)$$

As a result, the mean number of pairs  $\bar{N}_p$  oscillates [2]

$$\bar{N}_p(t) = \sinh^2(2\theta) \sin^2(\omega_B t) = \frac{U_s^2}{\hbar^2\omega_B^2} \sin^2(\omega_B t). \quad (12)$$

When  $q \gg U_s$ , the interactions are negligible, the frequency of the oscillation is trivially  $\omega_B \approx q/\hbar$  and their amplitude is  $(\bar{N}_p)_{\max} \approx U_s/q \ll 1$ . For  $U_s/N \ll q \ll U_s$ , the frequency of the oscillations  $\omega_B \approx \sqrt{2qU_s}/\hbar$  is modified by the interactions, and the amplitude  $[U_s/(2q)]^{1/2} \gg 1$  becomes substantial.

In order to verify these predictions, we measured the evolution of  $\bar{N}_p$  for various  $q$  (keeping  $q \ll U_s/N$ ,  $U_s$  and  $N$  are fixed). We fit the evolution with a sinusoidal function and report the value of the amplitude and of the period of the oscillation in figure 3. We observe a very good agreement with the Bogoliubov predictions.

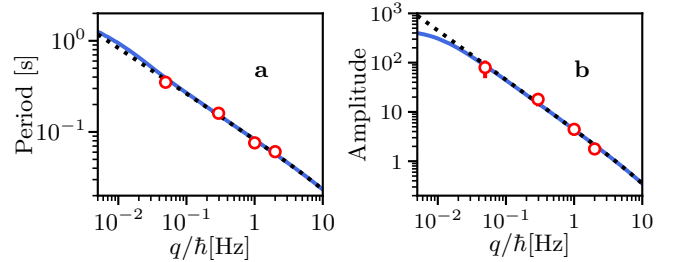

FIG. 3. Period (a) and amplitude (b) of the oscillation of  $\bar{N}_p$  in the reversible regime  $q \gg U_s/N$ . The red points are the experimental data, the solid lines are the results of a numerical resolution of the Schrödinger equation, and the dotted lines are given by the Bogoliubov approach.

## B. Generalized Gibbs ensemble

In the main text, we have used the GGE to describe the steady state reached in regime (iii), when  $q \ll U_s/N$  and relaxation occurs rapidly. More generally, numerical resolution of the Schrödinger equation reveals that at long times, relaxation always occurs, even in regime (ii), due to small deviations to the Bogoliubov approximation that makes the spectrum slightly non-linear. In that regime, we found numerically that the steady state verifies the predictions of the GGE computed using the Bogoliubov approximation. The constraint of vanishing magnetization [given in (9)] imposes the same number of excitations in each mode  $\hat{\alpha}$  and  $\hat{\beta}$ , such that the GGE density matrix can be written as

$$\rho \propto \sum_{N_{\text{ex}}} \frac{1}{(N_{\text{ex}}!)^2} (\hat{\alpha}^\dagger \hat{\beta}^\dagger)^{N_{\text{ex}}} |\text{vac}\rangle \langle \text{vac}| (\hat{\alpha} \hat{\beta})^{N_{\text{ex}}} \quad (13)$$

where the sum is taken over the states in a small energy window around the energy of the initial state  $E_i = U_s$ , i.e. with  $N_{\text{ex}} \approx \sinh^2(\theta)$ . Using Eq. (8) we find the number of pairs in the GGE steady state,

$$\langle \hat{N}_p \rangle_{\text{GGE}} = \frac{1}{2} \sinh^2(\theta) = \frac{U_s^2}{2\hbar^2 \omega_B^2}. \quad (14)$$

The damping of the oscillations takes a very long time when  $q \gg U_s/N$ . While relaxation proceeds, the system also undergoes atom losses due to collisions with the background gas, evaporation in the optical trap, or three-body relaxation. This forbids a direct experimental verification of prediction (14). However, we notice that in the Bogoliubov regime, the steady value of  $\bar{N}_p$  given by Eq. (14) is equal to half the amplitude of the initial oscillations of  $\bar{N}_p$ , given by Eq. (12). Based on this theoretical result, we analyze data taken in a broad range of magnetic field, from regime (i) to (iii), as follows:

- If we observe the relaxation of  $\bar{N}_p(t)$  within 500 ms, we directly measure the steady value.
- Otherwise, if we observe oscillations, we extract from a fit the time-average of  $\bar{N}_p(t)$ .

We report the results in figure 4 on a universal curve  $n_p = \bar{N}_p/N$  versus  $Nq/U_s$ . We found an excellent agreement with the predictions of the GGE over four orders of magnitude.

## III. CHAOTIC HAMILTONIAN

In the last section of the main text, we discuss the possibility to observe a chaotic behavior leading to thermalization. We introduce a modified Hamiltonian

$$\hat{H}' = q(\hat{N}_{+1} + \hat{N}_{-1}) + \frac{U_s}{2N} \hat{\mathbf{S}}^2 + \Omega \hat{S}_x, \quad (15)$$

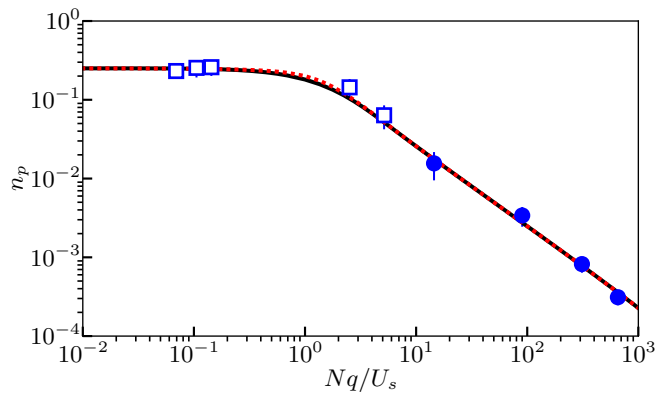

FIG. 4. Inferred steady-state values of the observable  $n_p$ , the mean fraction of  $m = \pm 1$  pairs. The blue circles are the average of oscillations observed in the reversible regime, where relaxation occurs on a time scale longer than the coherence time of our samples. For the blue squares, we observed relaxation on a shorter time scale and directly measured the steady state value of  $n_p$ . The red dashed line corresponds to the GGE prediction and the black solid line is the steady state extracted from a numerical resolution of the Schrödinger equation.

where

$$\hat{S}_x = \frac{1}{\sqrt{2}} \left[ \hat{a}_0(\hat{a}_{+1}^\dagger + \hat{a}_{-1}^\dagger) + \hat{a}_0^\dagger(\hat{a}_{+1} + \hat{a}_{-1}) \right], \quad (16)$$

is the  $x$  component of the collective spin.

Here, we briefly discuss a few important features of this Hamiltonian. It has also been studied in [3].

*a. Discrete symmetry :* The single-particle coupling term  $\propto \Omega$  in the Hamiltonian (15) breaks the  $\text{SO}(2)$  symmetry present in the original Hamiltonian (1). However, the discrete symmetry  $[\hat{H}', \hat{\mathcal{R}}] = 0$  is preserved, where

$$\hat{\mathcal{R}} = \exp(i\pi \hat{S}_x), \quad (17)$$

performs a rotation of angle  $\pi$  around the  $x$  axis.

The action of  $\hat{\mathcal{R}}$  in the basis of the collective spin-states is

$$\hat{\mathcal{R}}|S, M\rangle = (-1)^S |S, -M\rangle. \quad (18)$$

We recall that due to the exchange symmetry, the only possible states are those for which  $S$  and  $N$  have the same parity. We have  $\mathcal{R}^2 = \text{Id}$ , such that  $\mathcal{R}$  can have two eigenvalues  $(-1)^N$  and  $-(-1)^N$ , which we will refer to as even and odd parity, respectively. The eigenvectors with even parity are the states  $|S, 0\rangle$  and the symmetric superpositions

$$|\psi_{S,M}^+\rangle = \frac{1}{\sqrt{2}}(|S, M\rangle + |S, -M\rangle), \quad (19)$$

for  $M > 0$ . The dimension of the even-parity sector is thus  $(N/2 + 1)^2$ . The eigenvectors with odd parity are

the antisymmetric superpositions

$$|\psi_{S,M}^-\rangle = \frac{1}{\sqrt{2}}(|S,M\rangle - |S,-M\rangle), \quad (20)$$

with  $M > 0$ . They span a subspace of dimension  $(N/2) \times (N/2 + 1)$ . We call  $\hat{H}'_+$  (respectively,  $\hat{H}'_-$ ) the restriction of  $\hat{H}'$  to the even (resp. odd) parity sector.

*b. Numerical diagonalization :* To perform numerical computations, we first write  $\hat{H}'$  in the Fock state basis  $|N_0, M\rangle$  characterized by the three quantum numbers  $N$ ,  $N_0$  and  $M = N_{+1} - N_{-1}$ . We then perform the basis change

$$|N_0, \pm M\rangle \rightarrow \frac{1}{\sqrt{2}}(|N_0, M\rangle \pm |N_0, -M\rangle), \quad (21)$$

for  $M > 0$ . In the new basis,  $\hat{H}'$  is block diagonal and the blocks give directly  $\hat{H}'_{\pm}$ . We finally diagonalize  $\hat{H}'_{\pm}$  numerically to obtain the even- and odd-parity energies and eigenvectors separately.

*c. Level statistics :* In the chaotic regime achieved for instance when  $q/U_s = 0.8$  and  $\Omega/U_s = 0.6$ , the spectrum of  $\hat{H}'_{\pm}$  features level repulsion. The statistics of the level spacing is well reproduced by the Wigner-Dyson distribution, as shown for  $\hat{H}'_+$  in figure 3 of the main text (we find similar features for  $\hat{H}'_-$ ). For the full Hamiltonian  $\hat{H}'$ , approximate degeneracies between eigensates with opposite parity are possible due to the absence of coupling between the even and odd parity sectors. Without sorting the eigenvalues according to their parity, we do not observe the Wigner-Dyson distribution and level repulsion.

*d. Eigenstates thermalization* We show in figure 5 the diagonal matrix elements for the observables  $\hat{N}_0$  and  $\hat{S}_x^2$  in the basis of the even eigenstates of  $\hat{H}'$ . The ETH states that those matrix elements take comparable value for eigenstates sufficiently close in energy. We observe this behavior for both observables in the region A identified as chaotic in the main text. Outside this zone, the dispersion of the matrix elements increases, in particular for  $\hat{S}_x^2$ . These observations explain why we observed thermalization for a state in zone A and not for a state in B. We looked at other one- and two-body observables and always found that the ETH holds in the chaotic region of the spectrum. We also verified that it holds for eigenstates with odd parity.

*e. Dynamics* We focus on the dynamics of even-parity states obtained by a rotation around  $x$  of a polar BEC with each atom in  $|m = 0\rangle$ ,

$$|\psi_i(\theta)\rangle = \exp(-i\theta\hat{S}_x)|m = 0\rangle^{\otimes N}. \quad (22)$$

The parity of  $|m = 0\rangle^{\otimes N}$  is even and a rotation around  $x$  preserves the parity since the rotation operator commutes with  $\hat{\mathcal{R}}$ . In figure 3 of the main text, we show the

evolution of initial states with  $\theta = 0.6$  rad (blue, “non-chaotic” regime) and  $\theta = 1.2$  rad (red, “chaotic” regime).

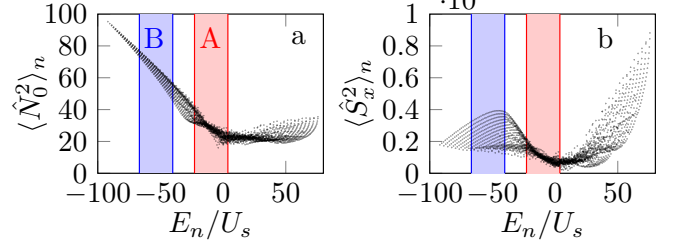

FIG. 5. Diagonal matrix elements of the observables  $\hat{N}_0$  (a) and  $\hat{S}_x^2$  (b) in the basis of the eigenstates of  $\hat{H}'$  with  $q = 0.8U_s$  and  $\Omega = 0.6U_s$ . The red and blue area correspond to the zones A and B introduced in the main text, and identified as chaotic and integrable, respectively. In zone A, eigenstates close in energy have similar expectation values for few body observables, in good agreement with the ETH. Outside this zone, we observe a larger dispersion, especially for  $\hat{S}_x^2$ .

#### IV. MEAN-FIELD APPROXIMATION

In a mean-field approximation, our system is described by a state  $|\zeta\rangle^{\otimes N}$ , where

$$|\zeta\rangle = \begin{pmatrix} \sqrt{n_{+1}}e^{i\phi_{+1}} \\ \sqrt{n_0} \\ \sqrt{n_{-1}}e^{i\phi_{-1}} \end{pmatrix} = \begin{pmatrix} \sqrt{\frac{1-n_0+m}{2}}e^{i\frac{\theta+\eta}{2}} \\ \sqrt{n_0} \\ \sqrt{\frac{1-n_0-m}{2}}e^{i\frac{\theta-\eta}{2}} \end{pmatrix}, \quad (23)$$

is a generic state for a spin-1 particle. In the following, to shorten the equations, we sometime use the variables  $n_{\pm 1}$  and  $\phi_{\pm 1}$ , but our set of independent variables is  $(n_0, \theta, m, \eta)$ . The mean-field energy per atom given the Hamiltonian (15) is (up to terms  $\sim 1/N$ )

$$E_s = -qn_0 + U_s \left[ n_0(1-n_0) + 2n_0\sqrt{n_{+1}n_{-1}}\cos\theta + \frac{m^2}{2} \right] + \Omega\sqrt{2n_0}(\sqrt{n_{+1}}\cos\phi_{+1} + \sqrt{n_{-1}}\cos\phi_{-1}). \quad (24)$$

The equations of motion can be derived starting from the Lagrangian density for the Schrödinger equation

$$\mathcal{L}(n_0, \theta, m, \eta, \dots) = \frac{i}{2}(\zeta^* \dot{\zeta} - c.c.) - E_s, \quad (25)$$

$$= -\frac{1-n_0}{2}\dot{\theta} - \frac{1}{2}m\dot{\eta} - E_s. \quad (26)$$

The Euler-Lagrange equations yield

$$\begin{aligned} \hbar\dot{n}_0 &= -2\frac{\partial E_s}{\partial\theta}, & \hbar\dot{\theta} &= 2\frac{\partial E_s}{\partial n_0}, \\ \hbar\dot{m} &= 2\frac{\partial E_s}{\partial\eta}, & \hbar\dot{\eta} &= -2\frac{\partial E_s}{\partial m}. \end{aligned} \quad (27)$$

After some algebra we arrive at

$$\hbar\dot{n}_0 = 4U_s n_0 \sqrt{n_{+1}n_{-1}} \sin \theta + \Omega \sqrt{2n_0} (\sqrt{n_{+1}} \sin \phi_{+1} + \sqrt{n_{-1}} \sin \phi_{-1}), \quad (28)$$

$$\begin{aligned} \hbar\dot{\theta} = & -2q + 2U_s(1 - 2n_0) + U_s \frac{(1 - n_0)(1 - 2n_0) - m^2}{\sqrt{n_{+1}n_{-1}}} \cos \theta \\ & + \Omega \left( \frac{2n_{+1} - n_0}{\sqrt{2n_0 n_{+1}}} \cos \phi_{+1} + \frac{2n_{-1} - n_0}{\sqrt{2n_0 n_{-1}}} \cos \phi_{-1} \right), \end{aligned} \quad (29)$$

$$\hbar\dot{m} = \Omega \sqrt{2n_0} (-\sqrt{n_{+1}} \sin \phi_{+1} + \sqrt{n_{-1}} \sin \phi_{-1}), \quad (30)$$

$$\hbar\dot{\eta} = U_s \frac{n_0 m}{\sqrt{n_{+1}n_{-1}}} \cos \theta - 2U_s m - 2p_z - \Omega \sqrt{\frac{n_0}{2}} \left( \frac{1}{\sqrt{n_{+1}}} \cos \phi_{+1} - \frac{1}{\sqrt{n_{-1}}} \cos \phi_{-1} \right). \quad (31)$$

### A. Integrable regime

Let us first consider the case  $\Omega = 0$ , describing a spin-1 BEC in a static magnetic field. From Eq. (30), we immediately see that  $m$  is constant, and that Eqs. (28,29) form a closed set of equations for the variables  $(n_0, \theta)$ . According to the Poincaré-Bendixson theorem, chaos cannot occur in this situation.

We also remark that  $n_0 = 1$  (implying  $n_{\pm 1} = 0$ ) is a solution of Eq. (28). The initial state for the experiment presented in Fig. 1 and Fig. 2 of the main text corresponds to  $n_0 = 1$ . Therefore, the dynamics that we observed cannot be captured within a mean-field approximation. More generally, regardless of the initial state, the solutions of Eqs. (28,29) are periodic when  $\Omega = 0$  [4], and thus incompatible with a relaxation of  $n_0$ .

### B. Chaotic regime

When the parameters  $U_s$ ,  $q$  and  $\Omega$  take comparable values, some regions of the phase space  $(n_0, \theta, m, \eta)$  become chaotic [3]. A convenient way to visualize chaotic trajectories relies on Poincaré sections, as shown in Fig. 6. We chose to look at the variables  $(n_0, \theta)$  when the trajectory crosses the subspace defined by  $m = 0$ . For the initial

state, we use  $\theta = \pi$ ,  $m = 0$ ,  $\eta = \pi/2$  and  $n_0 = 0.1$  (a) or  $n_0 = 0.6$  (b). The energies of those states, given by  $E_s = -qn_0$ , belong to the chaotic region A (a) or the regular one, B (b). We found that the region of quantum chaos identified by the energy level statistics (see main text) coincides with the region of classical chaos identified with Poincaré sections.

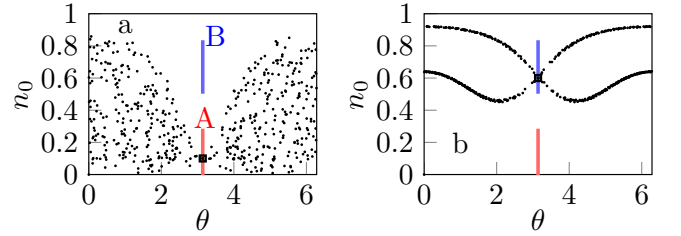

FIG. 6. Poincaré section  $(n_0, \theta)$  for the intersection surface  $m = 0$ . Here,  $q = 0.8U_s$  and  $\Omega = 0.6U_s$ . For our choice of initial state, with  $\theta = \pi$ ,  $m = 0$  and  $\eta = \pi/2$ , the energy is  $E_s = -qn_0$ . The red and blue lines indicate the energy windows A and B identified as chaotic and integrable in the main text, respectively. In (a) (resp. b) the initial state, shown by a dark square, corresponds to  $n_0 = 0.1$  (resp.  $n_0 = 0.6$ ) and belongs to zone A (resp. B). Accordingly, the Poincaré section spreads over a surface (resp. a line), and is characteristic of a chaotic (resp. regular) trajectory.

## V. POPULATIONS DISTRIBUTION FOR THE STATISTICAL ENSEMBLES

In this section, we derive the distribution  $P(N_0)$  of  $N_0$  for the microcanonical ensemble (ME) and for the generalized Gibbs ensemble (GGE). We focus on the situation where we observed relaxation, i.e. when we can neglect the quadratic Zeeman shift. In this case the Hamiltonian eigenstates are the collective spin states  $|S, M\rangle$ . The density matrix associated to the two ensembles are

$$\rho_{\text{ME}} \propto \sum_{E_S \in \mathcal{W}} \sum_{M=-S}^S |S, M\rangle \langle S, M|, \quad (32)$$

and

$$\rho_{\text{GGE}} \propto \sum_{E_S \in \mathcal{W}} |S, 0\rangle \langle S, 0|, \quad (33)$$

where the sums are taken over the spin manifolds whose energy  $E_S = S(S+1)U_s/(2N)$  sits in a window  $\mathcal{W}$  centered on the energy of the initial polar state  $E_i = U_s$ . The precise value of the width of the energy window is unimportant. In fact, we will see that all spin manifolds correspond to the same distribution  $P(N_0)$ , provided that the average over  $M$  for the ME, or a coarse-graining average for the GGE, are performed. It is thus sufficient to perform the calculation for the particular spin manifold with  $S^* \approx \sqrt{2N}$ , such that  $E_{S^*} = E_i$ .

### A. Preliminary

To obtain the desired distribution function, we need to compute the expansion of the collective spin states  $|S, M\rangle$  in the basis of Fock states  $|N_0, M\rangle$  with well-defined populations  $N_0$  and  $N_{\pm 1} = (N - N_0 \pm M)/2$ . To perform this calculation, it is convenient to introduce the overcomplete family of spin-nematic states  $|N : \mathbf{\Omega}\rangle = |m = 0\rangle_{\mathbf{\Omega}}^{\otimes N}$ , obtained as rotations of the polar state  $|m = 0\rangle_{\mathbf{\Omega}=\mathbf{e}_z}$ .

In the Fock basis, the spin-nematic states read

$$|N : \mathbf{\Omega}\rangle = \frac{1}{\sqrt{N!}} (\Omega_{+1} \hat{a}_{+1}^\dagger + \Omega_0 \hat{a}_0^\dagger + \Omega_{-1} \hat{a}_{-1}^\dagger)^N |\text{vac}\rangle, \quad (34)$$

with  $\Omega_{\pm 1} = \mp \frac{1}{\sqrt{2}} \sin \theta e^{\mp i\phi}$  and  $\Omega_0 = \cos \theta$ . Expanding the product, we have

$$|N : \mathbf{\Omega}\rangle = \sum_{N_0, M} (-1)^{N+1} f_{N_0}(\theta) e^{-iM\phi} |N_0, M\rangle. \quad (35)$$

with a coefficient

$$f_{N_0}(\theta) = \frac{1}{2^{\frac{N-N_0}{2}}} \sqrt{\frac{N!}{N_{+1}! N_0! N_{-1}!}} \cos \theta^{N_0} \sin \theta^{N-N_0}. \quad (36)$$

In the limit  $N \gg 1$ , these coefficients become narrow functions of  $\theta$  centered around the value  $\theta_0 \in [0, \pi/2]$ , such that

$$\sin \theta_0 = \sqrt{\frac{N - N_0}{N}}, \quad \cos \theta_0 = \sqrt{\frac{N_0}{N}}. \quad (37)$$

Using Stirling's formula and expanding the sinusoidal functions, we find that

$$f_{N_0}(\theta) \approx \frac{1}{\sqrt{2\pi}} \left( \frac{N}{N_{+1} N_0 N_{-1}} \right)^{1/4} e^{-\frac{M^2}{4(N-N_0)}} \left[ e^{-N(\theta-\theta_0)^2} + (-1)^{N_0} e^{-N(\theta+\theta_0-\pi)^2} \right]. \quad (38)$$

We use this approximate expression in actual calculations below.

Collective spin states and spin-nematic states are related by [5]

$$|S, M\rangle = \frac{1}{\sqrt{f_S^N}} \int_{\mathcal{S}} d^2 \mathbf{\Omega} Y_{SM}(\mathbf{\Omega}) |N : \mathbf{\Omega}\rangle. \quad (39)$$

Here the integral is taken over the unit sphere  $\mathcal{S}$ , the  $Y_{SM}$  are the spherical harmonics and the normalization factor is

$$f_S^N = \frac{4\pi 2^S N! (\frac{N+S}{2})!}{(\frac{N-S}{2})! (N+S+1)!} \approx \frac{4\pi}{N} e^{-\frac{S^2}{2N}}, \quad (40)$$

where the approximate expression holds for  $1 \ll S \ll N$ . Using  $|N : -\mathbf{\Omega}\rangle = (-1)^N |N : \mathbf{\Omega}\rangle$ ,  $Y_{SM}(-\mathbf{\Omega}) = (-1)^S Y_{SM}(\mathbf{\Omega})$ , and given that  $S$  and  $N$  have the same parity, we can restrict the integral over the upper hemisphere  $\mathcal{S}'$  of the unit sphere

$$|S, M\rangle = \frac{2}{\sqrt{f_S^N}} \int_{\mathcal{S}'} d^2 \mathbf{\Omega} Y_{SM}(\mathbf{\Omega}) |N : \mathbf{\Omega}\rangle. \quad (41)$$

## B. Generalized Gibbs Ensemble

For  $S \gg 1$  and  $M = 0$ , the spherical harmonics can be approximated by the leading term of their asymptotic expansion ,

$$Y_{S,0}(\mathbf{\Omega}) \approx \frac{(-1)^S}{\pi} \frac{\sin(S\theta + \frac{\pi}{4})}{\sqrt{\sin \theta}}. \quad (42)$$

We substitute Eqs. (35,38,42) in (41) and obtain after integration over  $\phi$

$$\langle N_0, 0 | S, 0 \rangle \approx \frac{4(-1)^{N_{+1}+S}}{\sqrt{\pi f_S^N}} \left( \frac{N}{N_0(N - N_0)^2} \right)^{1/4} \int_0^{\pi/2} d\theta \sqrt{\sin \theta} \sin \left( S\theta + \frac{\pi}{4} \right) \left[ e^{-N(\theta - \theta_0)^2} + (-1)^{N_0} e^{-N(\theta + \theta_0 - \pi)^2} \right]. \quad (43)$$

The integrand is sharply peaked on  $\theta_0$  and  $\pi - \theta_0$ . Since  $\theta_0 \in [0, \pi/2]$ , only the first term contributes significantly. Using a stationary phase approximation we obtain

$$\int_0^{\pi/2} d\theta \sqrt{\sin \theta} \sin \left( S\theta + \frac{\pi}{4} \right) e^{-N(\theta - \theta_0)^2} \approx \sqrt{\sin \theta_0} \operatorname{Im} \left[ e^{iS\theta_0 + \frac{\pi}{4}} \int_{-\infty}^{+\infty} d\theta e^{iS\theta} e^{-N\theta^2} \right] \quad (44)$$

$$= \sqrt{\frac{\pi}{N}} \sqrt{\sin \theta_0} \sin \left( S\theta_0 + \frac{\pi}{4} \right) e^{-\frac{S^2}{4N}}. \quad (45)$$

Using Eq. (40) and  $\sin \theta_0 = \sqrt{(N - N_0)/N}$ , we have

$$\langle N_0, 0 | S, 0 \rangle \approx (-1)^{N_{+1}+S} \frac{2}{\sqrt{\pi}} \frac{\sin(S\theta_0 + \frac{\pi}{4})}{[N_0(N - N_0)]^{1/4}}. \quad (46)$$

The associated probability distribution  $|\langle N_0, 0 | S, 0 \rangle|^2$  therefore oscillates very rapidly with  $N_0$  (recall that  $S \gg 1$ ) around a mean envelope function.

To extract this envelope (which is the experimentally relevant observable), we perform a coarse-graining average of the distribution  $P_{\text{GGE}}(\bar{N}_0)$  over an interval  $I = [\bar{N}_0 - \delta N_0, \bar{N}_0 + \delta N_0]$ ,

$$\bar{P}_{\text{GGE}}(\bar{N}_0) \approx \frac{4}{\pi} \frac{1}{2\delta N_0} \sum_{N_0 \in I} \frac{\sin^2(S\theta_0 + \frac{\pi}{4})}{[N_0(N - N_0)]^{1/2}}, \quad (47)$$

where the sum runs for  $N_0 \in I$  and of the same parity as  $N$  (thus,  $N_0$  varies by increment of 2). For  $N \gg 1$ , the discrete sum can be approximated by an integral over the variable  $x = (N_0 - \bar{N}_0)/N$ ,

$$\frac{1}{2\delta N_0} \sum_{N_0 \in I} \frac{\sin^2(S\theta_0 + \frac{\pi}{4})}{[N_0(N - N_0)]^{1/2}} \approx \frac{1}{4\delta x} \int_{-\delta x}^{+\delta x} dx \frac{\sin^2 \left( S\theta_0(x) + \frac{\pi}{4} \right)}{[(\bar{N}_0 + Nx)(N - \bar{N}_0 - Nx)]^{1/2}},$$

with  $\theta_0(x) \approx \bar{\theta}_0 - x/\sin(2\bar{\theta}_0)$  to first order in  $x$ . For a width  $\delta N_0 \ll N$  of the coarse-graining interval, the denominator is essentially constant and can be removed from the integral (this approximation breaks down on the edges of the distribution, where  $N_0 \sim \delta N_0$  or  $N_0 \sim N - \delta N_0$ ). Furthermore, if we choose  $\delta N_0 \gg N/S$ , *i.e.*  $\delta x \gg 1/S$ , the integration interval spans over several periods of the oscillating term in the numerator and this term averages to  $\approx 1/2$ . After coarse-graining, we thus obtain

$$\bar{P}_{\text{GGE}}(\bar{N}_0) \approx \frac{1}{\pi [\bar{N}_0(N - \bar{N}_0)]^{1/2}}. \quad (48)$$

As announced in the beginning, this formula holds without an average over  $S$ : it is valid for each individual  $|S, 0\rangle$  state with  $1 \ll S \ll N$ .

## C. Microcanonical ensemble

As for the GGE, we establish below that we do not need to average over a small energy window for the microcanonical ensemble as well, because the result for a given  $S$  actually does not depend on  $S$ . Thus, we consider for simplicity

the following density matrix, where  $S \sim \sqrt{2N}$  is fixed,

$$\rho_{\text{ME}} = \frac{1}{2S+1} \sum_{M=-S}^S |S, M\rangle \langle S, M|, \quad (49)$$

$$= \frac{4}{(2S+1)f_S^N} \iint_{S'} d^2\Omega_1 d^2\Omega_2 \sum_{M=-S}^S Y_{SM}(\Omega_1) Y_{SM}^*(\Omega_2) |N : \Omega_1\rangle \langle N : \Omega_2|, \quad (50)$$

$$= \frac{1}{\pi f_S^N} \iint_{S'} d^2\Omega_1 d^2\Omega_2 P_S(\Omega_1 \cdot \Omega_2) |N : \Omega_1\rangle \langle N : \Omega_2|, \quad (51)$$

where we have used the addition theorem for spherical harmonics, with  $P_S$  the Legendre polynomial of degree  $S$ . We want to compute

$$P_{\text{ME}}(N_0) = \frac{1}{\pi f_S^N} \iint_{S'} d^2\Omega_1 d^2\Omega_2 P_S(\Omega_1 \cdot \Omega_2) \sum_M \langle N_0, M | N : \Omega_1 \rangle \langle N : \Omega_2 | N_0, M \rangle, \quad (52)$$

where the sum runs over  $M \in [-(N - N_0), N - N_0]$ , with the same parity as  $N - N_0$ . We use the expressions (35,38), keeping only the terms that are significant in the upper sphere  $S'$ ,

$$P_{\text{ME}}(N_0) \approx \frac{1}{2\pi^2 f_S^N} \iint_{S'} d^2\Omega_1 d^2\Omega_2 P_S(\Omega_1 \cdot \Omega_2) \sum_M \left( \frac{N}{N_{+1}N_0N_{-1}} \right)^{1/2} e^{-\frac{M^2}{2(N-N_0)}} e^{-N(\theta_1-\theta_0)^2} e^{-N(\theta_2-\theta_0)^2} e^{-iM(\phi_1-\phi_2)}. \quad (53)$$

The dependence on  $M$  of  $N_{+1}N_{-1} = [(N - N_0)^2 - M^2]/4$  can be neglected because of the exponential factor cutting off terms with  $M$  larger than  $\sim \sqrt{N - N_0}$ . We can then evaluate the sum using a continuum approximation, valid for  $N_0, N - N_0 \gg 1$ ,

$$\sum_M e^{-\frac{M^2}{2(N-N_0)}} e^{-iM(\phi_1-\phi_2)} \approx \sqrt{\frac{\pi}{2}} (N - N_0) e^{-\frac{1}{2}(N-N_0)(\phi_1-\phi_2)^2}. \quad (54)$$

We now introduce the variables  $\varphi = \phi_1 - \phi_2$ ,  $\epsilon_{1,2} = \theta_{1,2} - \theta_0$ . The integral in Eq.(53) takes significant values for  $\varphi \sim 1/\sqrt{N - N_0}$  and  $\epsilon_{1,2} \sim 1/\sqrt{N}$ . As a result, we use the following approximations

$$\sin(\theta_{1,2}) \approx \sin(\theta_0) = \sqrt{(N - N_0)/N},$$

$$\Omega_1 \cdot \Omega_2 = \cos(\theta_0 + \epsilon_1) \cos(\theta_0 + \epsilon_2) + \sin(\theta_0 + \epsilon_1) \sin(\theta_0 + \epsilon_2) \cos(\varphi) \approx 1 - \frac{1}{2}(\epsilon_1 - \epsilon_2)^2 - \frac{1}{2} \sin^2 \theta_0 \varphi^2.$$

Introducing the variables  $\rho = \sqrt{\frac{1}{2}(\epsilon_1 - \epsilon_2)^2 + \frac{1}{2} \sin^2 \theta_0 \varphi^2}$ ,  $\gamma = \arctan[\sin \theta_0 \varphi / (\epsilon_1 - \epsilon_2)]$  and  $\epsilon = \epsilon_1 + \epsilon_2$  and using Eq. (54), Eq. (53) becomes

$$P_{\text{ME}}(N_0) \approx \sqrt{\frac{N}{N_0}} e^{\frac{S^2}{2N}} \int_0^{+\infty} d\rho \rho P_S(1 - \rho^2) e^{-N\rho^2}. \quad (55)$$

The last integral does not depend on  $N_0$ , and is thus a mere normalization factor. It can be computed by expanding the Legendre polynomials

$$P_S(1 - \rho^2) = \frac{1}{2^S} \sum_{k=0}^S \binom{S}{k}^2 (-\rho^2)^k (2 - \rho^2)^{S-k} \approx \sum_{k=0}^S \frac{S^{2k}}{k!^2} \frac{(-1)^k}{2^k} \rho^{2k}, \quad (56)$$

where we have used  $\rho^2 \lesssim 1/N$ , such that only the terms of the sum with  $k \sim 1$  are significant. We can then proceed to the integration

$$\int_0^{+\infty} d\rho \rho P_S(1 - \rho^2) e^{-N\rho^2} \approx \sum_{k=0}^S \frac{S^{2k}}{k!^2} \frac{(-1)^k}{2^k} \int_0^{+\infty} d\rho \rho^{2k+1} e^{-N\rho^2} \approx \sum_{k=0}^S \frac{S^{2k}}{k!^2} \frac{(-1)^k}{2^k} \frac{k!}{2N^{k+1}} \approx \frac{e^{-\frac{S^2}{2N}}}{2N}. \quad (57)$$

Inserting this expression into Eq. (55), we finally arrive at

$$P_{\text{ME}}(N_0) \approx \frac{1}{2\sqrt{NN_0}}. \quad (58)$$

Let us again remark that we did not use any average over  $S$  in order to derive this formula, and we only assumed  $1 \ll S \ll N$ . This ensures the equivalence between the microcanonical and canonical ensembles. We also point out that the distribution  $P_{\text{ME}}(N_0)$  is smooth without the need for coarse-graining, in contrast with the GGE.

- 
- |                                                                                      |                                                                                                           |
|--------------------------------------------------------------------------------------|-----------------------------------------------------------------------------------------------------------|
| [1] T.-L. Ho, Phys. Rev. Lett. <b>81</b> , 742 (1998).                               | 053604 (2020).                                                                                            |
| [2] G. I. Mias, N. R. Cooper, and S. Girvin, Phys. Rev. A <b>77</b> , 023616 (2008). | [4] W. Zhang, D. L. Zhou, M.-S. Chang, M. S. Chapman, and L. You, Phys. Rev. A <b>72</b> , 013602 (2005). |
| [3] M. Rautenberg and M. Gärttner, Phys. Rev. A <b>101</b> , 053604 (2020).          | [5] R. Barnett, J. D. Sau, and S. D. Sarma, Physical Review A <b>82</b> , 031602 (2010).                  |
